# Supplementary material for: Decision-Oriented Dialogue for Human-AI Collaboration
Source: arXiv:2305.20076 source file (2024-05-05)
Supplement: Supplementary file 1 [file matching.tex]

\begin{figure}[H]
    \centering
    \setlength{\fboxrule}{1pt}
    \setlength{\fboxsep}{0pt}
    \fcolorbox{black}{white}{%
      \includegraphics[width=.48\textwidth]{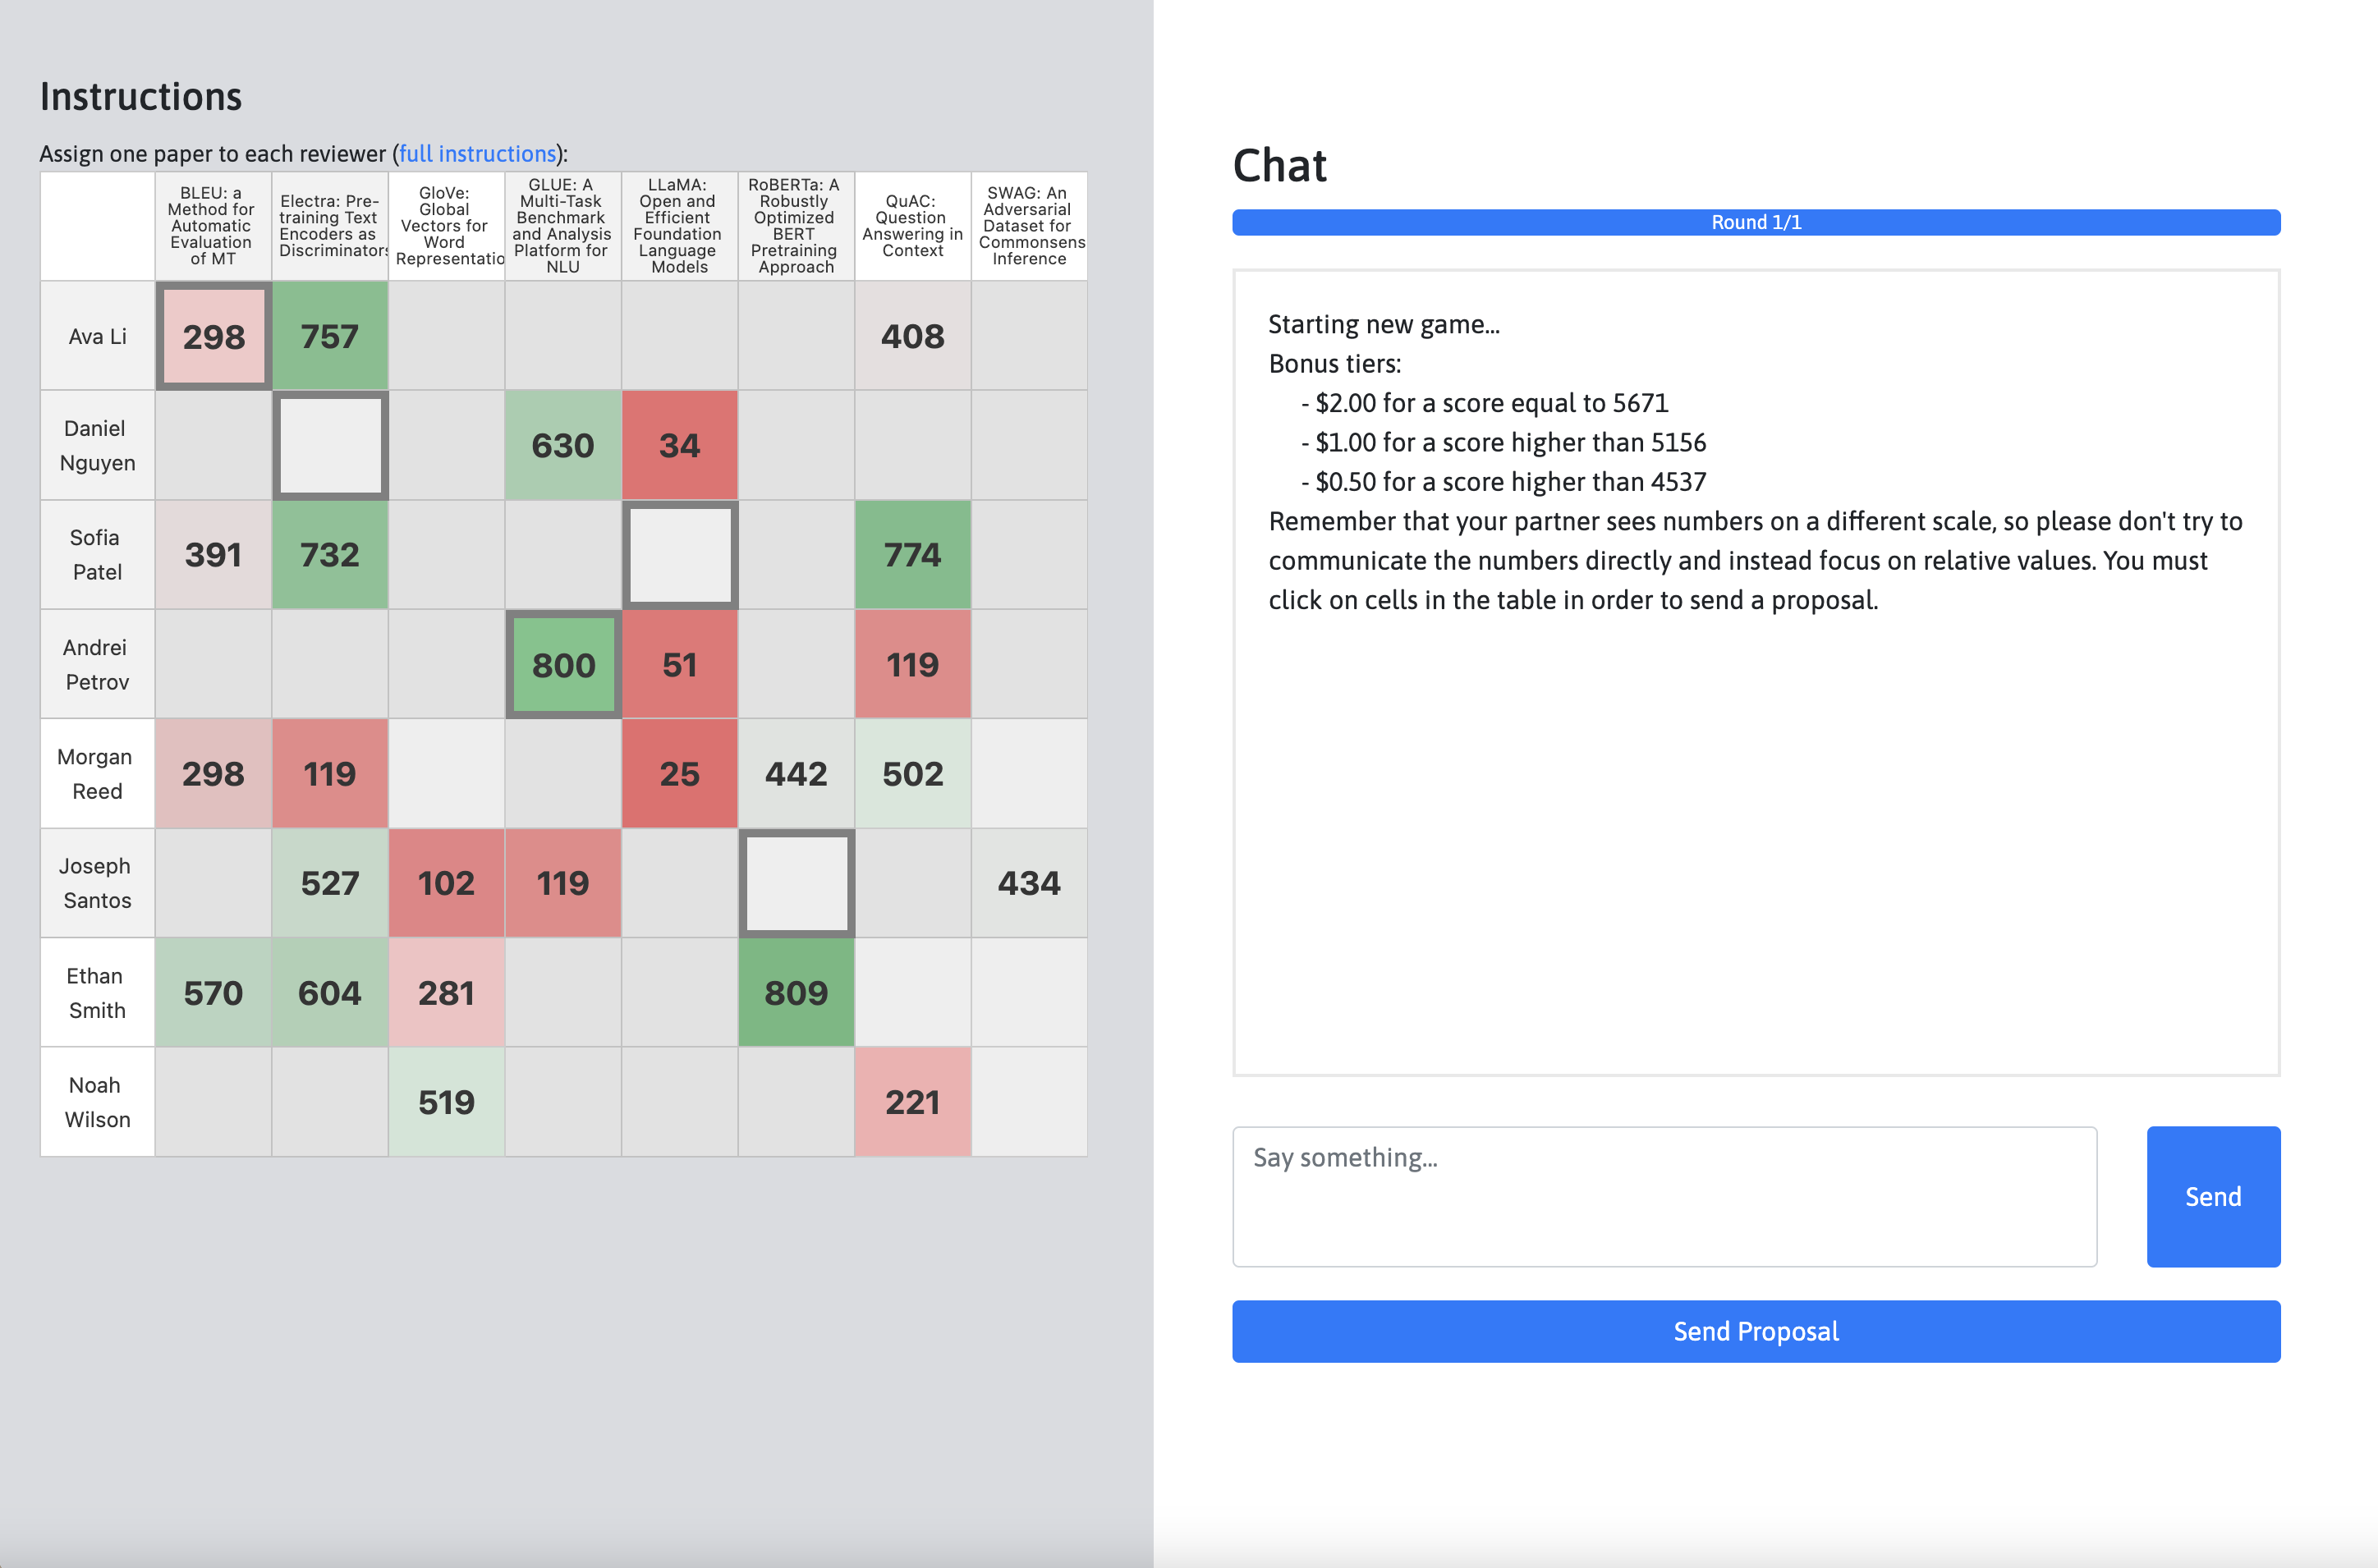}%
    }
  \caption{UIs for both players in the \texttt{Optimization} task. Both players observe a subset of reviewer-paper affinities in a spreadsheet table. They can send proposals by clicking on cells in the table, at which point the proposal appears in the other player's table.}
  \label{fig:matching-interface}
\end{figure}
